# Supplementary material for: Rethink the Role of Deep Learning towards Large-scale Quantum Systems
Source: arXiv:2505.13852 source file (2025-05-20)
Supplement: Supplementary file 1 [file cnn.tex]

\begin{table}[]
    \centering
    \begin{tabular}{c|c}
        Layer & Settings \\
        Convolutional layer &  \\
        Activation layer & ReLU\\
        Dropout & \\
        Fully connected layer & \\
        Activation layer & ReLU\\ 
        Fully connected layer & \\ 
        Dropout & \\ 
    \end{tabular}
    \caption{Model architecture of Couvolutional Neural Network for QSL tasks}
    \label{tab:cnn_arch}
\end{table}
