# Supplementary material for: Rethink the Role of Deep Learning towards Large-scale Quantum Systems
Source: arXiv:2505.13852 source file (2025-05-20)
Supplement: Supplementary file 2 [file mlp.tex]

\begin{table}[h]
    \centering
    \begin{tabular}{c|c}
        \toprule
      Layer &  Settings\\
      \midrule
        Fully connected layer & $D_{\text{in}}\times 128$ units\\
        Activation layer & ReLU \\
        Dropout & $p=0.5$ \\
        Fully connected layer & $128 \times D_{\text{out}}$ \\
        \bottomrule
    \end{tabular}
    \caption{Model architecture of MLP for QSL models}
    \label{tab:mlp_arch}
\end{table}
